# Supplementary material for: Hotter isn't faster for a melting RNA hairpin
Source: arXiv:2411.03072 source file (2024-11-05)
Supplement: Supplementary file 1 [file Supplementary_Material.pdf]

# Supplementary Materials for “Hotter isn’t faster for a melting RNA hairpin”

Huaping Li,<sup>1</sup> E. M. Bahçeci,<sup>2</sup> M. Sayar,<sup>3</sup> and A. Kabakcıoğlu<sup>4,\*</sup>

<sup>1</sup>Wenzhou Institute, University of Chinese Academy of Sciences, Wenzhou, Zhejiang 325001, China

<sup>2</sup>Processing and Performance of Materials, Department of Mechanical Engineering,  
Eindhoven University of Technology, 5600 MB Eindhoven, Netherlands

<sup>3</sup>College of Engineering, Koç University, Istanbul, 34450, Türkiye

<sup>4</sup>College of Sciences, Koç University, Istanbul, 34450, Türkiye

## A. The coarse-grained hairpin model

The RNA hairpin model features two specifically complementary strands that are clamped at one end (see Fig. 1). Each strand is depicted as a bead-spring chain, where each bead represents a base which is free to move in three dimensions subject to the gradient and stochastic forces. The overall potential energy of the system can be expressed as the sum of four components:

$$V = V_b + V_{bp} + V_a + V_{dih} \quad (1)$$

The force field we use is a minimal model which com-

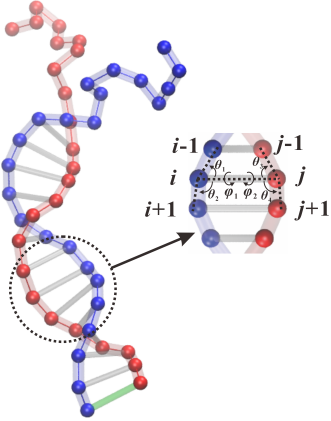

FIG. 1. Coarse-grained hairpin model. Red and blue beads represent the complementary bases on the two strands, respectively, while shaded strips illustrate the nucleotide chains. The base pairs are indicated by gray sticks, and the clamping bond is depicted by green stick. Symbols related to non-bonded interactions are also marked in the figure.

prises five parameters with units of length dictated by the geometry of the helical structure, four spring constants whose magnitudes determine the elastic properties and reflect the progressively increasing stiffness associated with dihedral torsion, angle bending and bond stretching, and three energy parameters which set the depth of each potential well relative to the unbound state, ultimately determining the denaturation conditions.

Within each strand, adjacent bases are linked by a harmonic bond with an equilibrium bond length of  $b_0$ .

$$V_b(b) = K_b(b - b_0)^2 \quad (2)$$

The hydrogen bonds between complementary beads across the strands are represented using a piecewise potential, composed of the attractive cosine function and the repulsive harmonic function that are joint at the equilibrium distance,  $d_0$ .

$$V_{bp}(d) = \begin{cases} K_{bp}(d - d_0)^2 - \varepsilon_{bp}, & d < d_0 \\ -\varepsilon_{bp}f(d), & d_0 \leq d < d_{max} \\ 0, & d_{max} \leq d \end{cases} \quad (3)$$

Here,  $f(d) = 0.5[1 + \cos(\frac{d-d_0}{d_{max}-d_0}\pi)]$  is a smooth function over the interval  $[d_0, d_{max}]$  where the complementary bases attract each other.

The native structure of the duplex is preserved through inter-strand (two-bond) angle interactions and (three-bond) dihedral interactions,

$$V_a(\theta) = K_a(\cos \theta - \cos \theta_0)^2 - \varepsilon_a, \quad (4)$$

$$V_{dih}(\varphi) = K_{dih}[1 - \cos(\varphi - \varphi_0)] - \varepsilon_{dih}, \quad (5)$$

in the case of  $d < d_0$ . When the hydrogen bond distance is between  $d_0$  and  $d_{max}$ , the smooth transition function,  $f(d)$ , is multiplied to Eq.4 and 5 to account for the distance dependence of inter-strand interactions.

Additionally, excluded-volume interactions are applied between nonadjacent intra-strand bases and inter-strand bases. Model parameters are listed in Table I below.

TABLE I. Model parameters.

| $K_b$ | $b_0$ | $K_{bp}$ | $\varepsilon_{bp}$ | $K_a$ | $\theta_0$ | $\varepsilon_a$ | $K_{dih}$ | $\varphi_0$ | $\varepsilon_{dih}$ | $d_0$ | $d_{max}$ |
|-------|-------|----------|--------------------|-------|------------|-----------------|-----------|-------------|---------------------|-------|-----------|
| 200   | 1.0   | 100      | 1.0                | 5.0   | 1.387      | 0.1             | 1.0       | 1.832       | 0.1                 | 2.14  | 2.34      |

In summary, the model consists of two single-stranded backbone chains connected by hydrogen bonds. Subsequent bases along each backbone are connected by unbreakable harmonic bonds with an equilibrium length  $b_0$  and rotationally free joints at bead positions. Bases in opposite strands are allowed to form (breakable) hydrogen bonds with their complementary base only, through

\* akabakcioglu@ku.edu.tr

a segmented potential with a minimum value of  $-\varepsilon_{bp}$ , a pair distance of  $d_0$ , and a maximum distance of  $d_{max}$ . Pairing also induces inter-strand angle and dihedral potentials, yielding the helical structure of the duplex.

The MD simulations of the model were performed using in-house software implemented in C/C++. This software employs coarse-grained MD with Langevin dynamics to simulate RNA hairpin models in an NVT ensemble. The initial structures were constructed as double-stranded helices in the folded state brought to thermal equilibrium below the critical temperature ( $T_m$ ). We then immediately transferred the system to an environment with a temperature exceeding  $T_m$ , enabling the hairpin structures to fully denature until all base pair interactions were disrupted. To systematically examine the melting behavior of the hairpin structures, we explored a parameter space encompassing chain lengths of 40, 80, 120, 160, 240, 320, and 640, and temperatures ranging from 0.175 to 0.210 in units of the base pair binding energy  $\varepsilon_{bp}$ . For each unique combination of chain length and temperature, we conducted 100 independent simulations to acquire a sufficient number of trajectories for comprehensive analysis and to reliably calculate the average melting time.

For accurate identification of the melting temperature, we also generated equilibrated single-stranded structures in the denatured state, in order to run folding simulations at varying temperatures. The melting curves were obtained by ensuring that the melting and folding simulations starting from opposite ends reach the same denaturation fraction for a given temperature, in order to avoid any bias due to insufficient equilibration times.

### B. Determining the crossover temperature

Kymographs for individual trajectories of the 100 samples for  $L = 640$  at three temperatures corresponding to type-Y ( $T = 0.176$ ), type-X ( $T = 0.195$ ) and the crossover ( $T = 0.179$ ) regimes (Figure 2) allow an in-depth exploration of each melting regime. In each kymograph, the bound base pairs in the duplex region are shown in blue, and the denatured regions on the two ends of the duplex are shown in white. Note that, the horizontal time axis is normalized for each kymograph to fit in the grid structure.

The crossover boundary separating type-X and type-Y melting regimes is most easily identified by considering the statistics of melting times. A balanced mixture of type-X and type-Y trajectories, as shown in Fig.2b above, implies a wide spread of denaturation times. After some investigation, we observed that the ratio of the standard deviation to the mean,  $std(\tau_m)/\langle\tau_m\rangle$ , known as the “coefficient of variation” (CV) depends weakly on the length away from the crossover in each regime and peaks in between. We therefore defined the crossover temperature as the temperature at which CV reaches its maximum value.

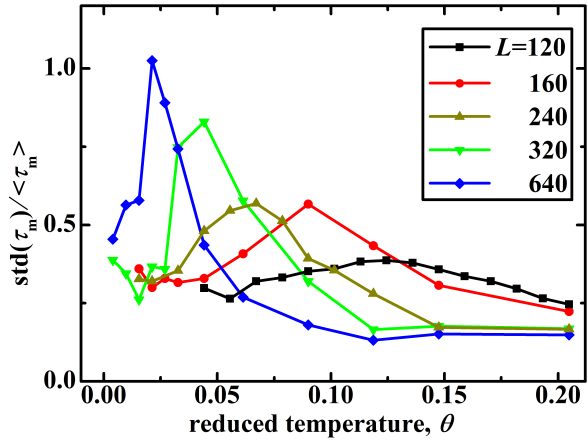

FIG. 3. Coefficient of variation of the denaturation time *vs.* temperature for different RNA hairpin lengths.

Fig.3 shows the change in CV along each temperature scan given in Fig.2b of the main text. Note that the peak in CV is sharper for longer chains as the gap between the melting times of type-X and type-Y trajectories widens and the non-monotonicity of the mean melting time *vs.* temperature gets more pronounced (see the main text).

### C. Duplex rotation during denaturation

We argue in the main text that the X-Y crossover occurs as a consequence of the communication between the two ends of the molecule mediated by the rotation of the duplex. In order to check that duplex rotation—rather than the rotation of tail segments—is the dominant response to pair breaking, we calculated the mean angular velocity of the duplex about its central axis during the denaturation process. Fig.4 shows that the duplex rotation sets in after an initial transient during which  $\leq 10\%$  of the molecule has denatured. The saturation value of the rotation angle per broken base pair in Fig.4 corresponds to the stacking angle  $2\pi/\lambda$  of the duplex, where  $\lambda = 10.5$  is the pitch of the helix, attesting to the fact that the twist of the denatured portion is essentially relaxed by duplex rotation. A comparison of data from different molecule sizes also reveals that the transient period gets relatively shorter for longer chains, providing further support for the proposed phenomenological framework in view of the fact that X-Y crossover is more prominent in relatively longer molecules.

### D. Selection of type-X and type-Y trajectories

The scaling of the denaturation time with length was investigated separately for both regimes. This analysis requires labeling individual trajectories as type-X or type-Y. As evident from Fig.2, this can be challenging

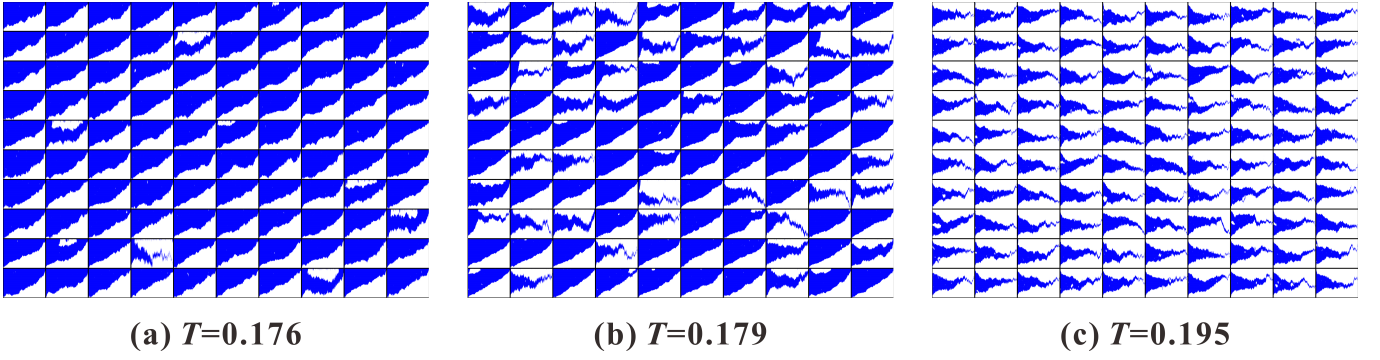

FIG. 2. Kymographs for the trajectories used in the paper, for selected temperatures corresponding to (a) type-Y; (b) crossover; (c) type-X melting regimes.

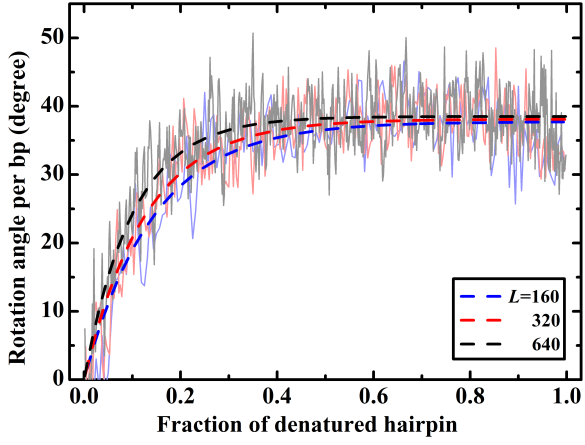

FIG. 4. Rotation angle of the duplex segment during type-Y melting process measured on hairpins with different lengths. Note that the duplex rotation sets in relatively earlier in longer molecules.

for some trajectories. We therefore developed an analytical approach based on the size of the white areas above ( $A_{head}$ ) and below ( $A_{tail}$ ) the blue regions in the kymographs which, respectively, correspond to the lengths of the denatured regions at the two ends of the molecule integrated over time. For type-Y denaturation starting from the tail, the ratio  $A_{tail}/A_{head}$  is significantly larger than unity since the head remains bound except for small fluctuations. In contrast, the competition of the two y-junctions characteristic of type-X trajectories

yields a ratio close to unity. Accordingly, the distribution of the quantity  $r \equiv \log_{10}(A_{tail}/A_{head})$  shown in Fig.5, calculated using trajectories at different temperatures and lengths, displays two distinct peaks, one with a mean around  $r = 0$ , and one around  $r = 4$ , providing further evidence for the presence of two distinct denaturation pathways and for the adequacy of the ratio  $r$  as a classification measure.

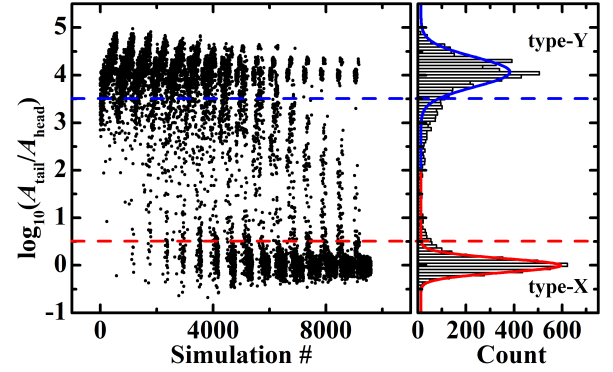

FIG. 5. Distribution of  $\log_{10}(A_{tail}/A_{head})$  defined in the text, derived from denaturation trajectories at different temperatures and molecule sizes. The two thresholds used for selecting type-X and type-Y trajectories are shown by the dashed lines in red and blue, respectively.

Using empirically determined thresholds, we labeled trajectories with  $r \geq 3.5$  as type-Y and those with  $r \leq 0.5$  as type-X. The quality of the two sets was then visually inspected for further validation.
